# Supplementary material for: Convergence Rate Analysis of Proximal Iteratively Reweighted $\ell_1$ Methods for $\ell_p$ Regularization Problems
Source: arXiv:2007.05747 source file (2021-01-11)
Supplement: Supplementary file 1 [file appendix.tex]

\section*{Appendix}

Proof of \cref{lem.c123}.

\begin{proof}  
  For simplicity and without loss of generality,  we can assume $\mathbb{R}^{\Ical^*}= \mathbb{R}^n$, so that
   the components of $\{x^k\}_{k>K}$ are all uniformly bounded away from 0 and that 
$w(x_i^k, \epsilon_i^k) \le C/\lambda$ for all $i$ and $k > K $, meaning 
\begin{equation}
\label{tmp.w bound}
|x_i^k|+(\delta_i^k)^2 \ge \left( \frac{p\lambda}{C}\right)^{\frac{1}{1-p}}.
\end{equation}

	\textbf{C1.}
	From \eqref{eq:convergence4}, we have for any $k\in \mathbb{N}$,
%	\[   F(z^k)- F(z^{k+1}) \geq  (M-\frac{L_f}{2})\|x^{k+1}-x^k\|^2_2. \]
%	It then follows that 
	\begin{equation}\label{eq:kl1}
	\begin{aligned}
& \ F(z^k)-F(z^{k+1}) \\
=&\  F(x^{k},\delta^{k})-F(x^{k+1},\delta^{k})+F(x^{k+1},\delta^{k})-F(x^{k+1},\delta^{k+1})\\
	 \geq &\  (M-\frac{L_f}{2})\|x^{k+1}-x^k\|^2_2+F(x^{k+1},\delta^{k})-F(x^{k+1},\delta^{k+1}). 
%	 \geq &\  (M-\frac{L_f}{2})\|x^{k+1}-x^k\|^2_2 +  \lambda\sum_{i=1}^n [ (|x^{k+1}_i|+(\delta^{k}_i)^2 )^p - (|x^{k+1}_i|+(\delta^{k+1}_i)^2 )^p]
	 \end{aligned}
	 \end{equation}
%	 Therefore, it suffices to show that $F(x^{k+1},\delta^{k})-F(x^{k+1},\delta^{k+1}) \ge C \|\delta^{k+1} - \delta^k\|_2^2$ for 
%	 some constant $C>0$. 
%	 :=&\ C_1 \|x^{k+1}-x^k\|^2_2 + F(x^{k+1},(\delta^{k})^2 )-F(x^{k+1},(\delta^{k+1})^2)
%	 	\end{aligned}
%	 \end{equation}
Now we investigate $F(x^{k+1},\delta^{k})-F(x^{k+1},\delta^{k+1})$. 
	  According to Taylor's theorem,  there exists $c_i^{k+1} \in [ \delta_i^{k+1}, \delta_i^{k}]$ for each $i$ such that
	 \begin{equation}\label{eq:kl2}
	 \begin{aligned}
	   F(x^{k+1},\delta^{k})-F(x^{k+1},\delta^{k+1})
	  = & \lambda \sum_{i=1}^n  (|x^{k+1}_i|+(\delta_i^{k})^2)^p-(|x^{k+1}_i|+(\delta_i^{k+1})^2)^p\\
	  = &\lambda \sum_{i=1}^n   2pc_i^{k+1}(|x_i^{k+1}|+  (c_i^{k+1})^2)^{p-1}(\delta_i^k-\delta_i^{k+1}). 
	  \end{aligned}
	 \end{equation}
%	 So, we can get the relation between   $F(x^{k+1},(\delta^{k})^2 )-F(x^{k+1},(\delta^{k+1})^2)$ and $\|\delta^{k}-\delta^{k+1}\|^2$.
%	 \begin{equation*}
%	 \begin{aligned}
%	 F(x^{k+1},(\delta^{k})^2 )-F(x^{k+1},(\delta^{k+1})^2)
%	&= \lambda \sum_{i=1}^{n}[(|x^{k+1}_i|+(\delta_i^{k})^2)^p-(|x^{k+1}_i|+(\delta_i^{k+1})^2)^p]\\
%	&= 2\lambda\sum_{i=1}^{n} pc_i^{k+1}(|x_i^{k+1}|+c_i^2)^{p-1}(\delta_i^k-\delta_i^{k+1})\\ 
%	\end{aligned}
%	\end{equation*}
%	It follows from the boundedness of  $\{x^k\}$  by \cref{prop.sign}   
%	that the weights $\{w_i^k\}$ are all bounded away from 0.
	% In fact, b
	 By  \cref{prop.sign},  for each component and any $k$,  we have    
	\begin{equation*}
 	(|x_i^{k}|+\epsilon_i^k)^p \leq \sum_{i=1}^{n}(|x_i^{k}|+\epsilon_i^k)^p 
	\leq F(x^0,\epsilon^0) - f(x^k) \leq F(x^0,\epsilon^0) - \underline{f}.
 	\end{equation*}
Accordingly, a lower bounded of weights, denoted by $\underline{w}$, can be given by 
	\[
	w(x_i^k, \epsilon_i^k)= p(|x_i^k|+\epsilon_i^k)^{p-1} \geq \underline{w}: = p(F(x^0,\epsilon^0) - \underline{f})^{\frac{p-1}{p}}.
	\]
	It then follows from \eqref{eq:kl2} that 
	\begin{equation}
	\label{eq:mykl2}
	\begin{aligned}
	 F(x^{k+1},\delta^{k})-F(x^{k+1},\delta^{k+1}) \ge &  2 \lambda \underline{w}  \sum_{i=1}^{n} \delta_i^{k+1}(\delta_i^k-\delta_i^{k+1})\\
	 \ge &  \  2 \lambda \underline{w}  \frac{\sqrt{\mu} }{1-\sqrt{\mu}}  \sum_{i=1}^{n} (\delta_i^k-\delta_i^{k+1})^2,
	 \end{aligned}
	 \end{equation} 
 where the second inequality is from 
 	$ \delta_i^{k+1} = \frac{\sqrt{\mu} }{1-\sqrt{\mu}}(\delta_i^k-\delta_i^{k+1})$ due to 
	 $\epsilon^{k+1}_i =   \mu\epsilon^{k}_i$. 
	 
%	 , we have  
%%	Otherwise, it holds that $\epsilon_i^{k+1} = \epsilon_i^k$, 
%     meaning 
%	$ \delta_i^{k+1}(\delta_i^k-\delta_i^{k+1}) =  \frac{\sqrt{\mu} }{1-\sqrt{\mu}} (\delta_i^k-\delta_i^{k+1})^2$. 
%		Overall, we have from \eqref{eq:mykl2} that 
%	\[  F(x^{k+1},\delta^{k})-F(x^{k+1},\delta^{k+1}) \ge 2 \lambda \underline{w}  \frac{\sqrt{\mu} }{1-\sqrt{\mu}}
%	  \sum_{i=1}^{n} (\delta_i^k-\delta_i^{k+1})^2 .
%	  \]  
Combining  \cref{eq:kl1} and \eqref{eq:mykl2}, we obtain that
	\[
	F(z^k)-F(z^{k+1}) \geq a \|x^{k+1}-x^k\|^2_2 + a \|\delta^{k+1}-\delta^k\|^2_2 \geq a\|z^k-z^{k+1}\|^2_2
	\]
	with $a:=\min\{(M-\frac{L_f}{2}),  2 \lambda \underline{w}  \frac{\sqrt{\mu} }{1-\sqrt{\mu}}\}$, completing the proof of 
		\textbf{C1.}
%	
%	
%	 So, we have
%	\begin{equation}\label{eq:kl3}
%	\begin{aligned}
%	 F(x^{k+1},(\delta^{k})^2 )-F(x^{k+1},(\delta^{k+1})^2) &\geq  2 \lambda\sum_{i=1}^{n} \underline{w} c_i^{k+1}(\delta_i^k-\delta_i^{k+1})\\
%	&\geq 2 \lambda\sum_{i=1}^{n} \underline{w} \delta_i^{k+1}(\delta_i^k-\delta_i^{k+1})\\
%	&= 2 \lambda \underline{w} \frac{\sqrt{\mu} }{1-\sqrt{\mu} }\sum_{i=1}^{n} (\delta_i^k-\delta_i^{k+1})^2\\
%	&:= C_2 \|\delta^k-\delta^{k+1}\|^2
%	\end{aligned}
%	\end{equation}

	\textbf{C2.}  
	  	The gradient of $F$ with respect to $z$ at $z^{k+1}$ can be computed  as:
	\[\left\{\begin{aligned}
	\nabla_x F(x^{k+1},\delta^{k+1}) = & \nabla f(x^{k+1}) + \lambda   w^{k+1}\circ \text{sign}(x^{k+1}), \\
	 \nabla_{\delta} F(x^{k+1},\delta^{k+1}) = & 2\lambda w^{k+1}\circ \text{sign}(x^{k+1}) \circ \delta^{k+1}.
	\end{aligned}\right.
	\]
	 Suppose $x^{k+1}$ is the optimal solution of minimizing $G(x;x^k,\epsilon^k)$,  then we have 
	\[
	0 = \nabla f(x^k) + B^k(x^{k+1}-x^k)+ \lambda  w^{k}\circ \text{sign}(x^{k+1}).
	\]
	It follows that 
	\begin{equation*}\label{eq:kl4}
	\begin{aligned}
	&\ \|\nabla f(x^{k+1}) + \lambda  w^{k+1}\circ \text{sign}(x^{k+1})  \|_2\\
	= &\ \|\nabla f(x^k)-\nabla f(x^{k+1}) + B^k(x^{k+1}-x^k)+ \lambda ( w^k-w^{k+1})\circ \text{sign}(x^{k+1} )\|_2\\
	 \leq  &\ \|\nabla f(x^k)-\nabla f(x^{k+1})\|_2 + \| B^k(x^{k+1}-x^k)\|_2 +\lambda \|w^k-w^{k+1}\|_2\\
	 \leq &\ L_f\|x^k-x^{k+1}\|_2 + M\|x^{k+1}-x^k\|_2 + \lambda \|w^k-w^{k+1}\|_2 \\
	\leq &\ (L_f + M)\|x^{k+1}-x^k\|_2 +\lambda  \| w_i^k-w_i^{k+1}\|_1,
	\end{aligned}
	\end{equation*}	
	where the second inequality is by Assumption \ref{ass.basic}. 
	We now investigate  $\| w_i^k-w_i^{k+1}\|_1$.   It follows that for each $i$ there exists 
	$c\in [|x^{k+1}_i|+(\delta_i^{k+1})^2, |x^{k}_i|+(\delta_i^{k})^2]$ such that 
		\begin{equation*}
	\begin{aligned}
	|w_i^k-w_i^{k+1}| &=   p|(|x^{k+1}_i|+(\delta_i^{k+1})^2)^{p-1}-(|x^{k}_i|+(\delta_i^{k})^2)^{p-1}|  \\
	&= p|(p-1)c^{p-2}(|x^{k+1}_i|+(\delta^{k+1})^2 -|x^{k}_i|-(\delta_i^{k})^2 )|\\
	&\leq p(1-p)c^{p-2}\left( |x_i^{k+1}-x_i^k| +  |(\delta_i^{k+1})^2-(\delta_i^{k})^2|\right)\\
		&= p(1-p)c^{p-2}\left( |x_i^{k+1}-x_i^k| +  (\delta_i^{k+1} + \delta_i^k)(\delta_i^{k} - \delta_i^{k+1})\right)\\
	&\leq p(1-p)  \left( \frac{p\lambda}{C}\right)^{\frac{p-2}{1-p}} (|x_i^{k+1}-x_i^k|+2\delta_i^0|\delta_i^{k+1}-\delta_i^{k}| ),
   % &:= D_1 (|x_i^{k+1}-x_i^k|+2\delta_i^0|\delta_i^{k+1}-\delta_i^{k}| )
	\end{aligned}
	\end{equation*}
	where the last equality is by the fact that $\{\delta_i^k\}$ is monotonically decreasing, and the last inequality is by \eqref{tmp.w bound}.
	Hence 
	\[ \|w^k-w^{k+1}\|_1 \le \lambda   p(1-p)  \left( \frac{p\lambda}{C}\right)^{\frac{p-2}{1-p}} \sqrt{n} \left(\|x^k-x^{k+1}\|_2 + 2\|\delta^0\|_\infty \|x^k-x^{k+1}\|_2 \right).\]
	This combined with \eqref{eq:kl4} yields 
	\begin{equation}\label{eq:kl5} 
	\begin{aligned}
	\|\nabla_xF(z)\|_2 = &\ \|\nabla f(x^{k+1}) + \lambda  w^{k+1}\circ \text{sign}(x^{k+1})  \|_2\\
	   \le &\  	 C_1 \left( \| x^{k+1}-x^k\|_2 +  \|\delta^{k+1}-\delta^{k}\|_2 \right)
	   \end{aligned}
	 \end{equation}
with \[C_1 : =\max\left(   L_f + M +     \lambda   p(1-p) \sqrt{n}  \left( \frac{p\lambda}{C}\right)^{\frac{p-2}{1-p}},  2  \lambda   p(1-p) \sqrt{n}  \left( \frac{p\lambda}{C}\right)^{\frac{p-2}{1-p}}     \|\delta^0\|_\infty   \right). \]

%	
%	 because we know that if $w(x_i^{\bar k}, \epsilon_i^{\bar k}) > C/\lambda$ % \ \text{ or } \  |x_i^k| <  \ \text{ or } \  \epsilon_i^k<?\]
%	for some ${\bar k}\in \mathbb{N}$,  then  $i\in\Acal^*$. So, we can choose a constant $\bar{w}>C/\lambda$ as a upper bound of $w$, we set all $w=\bar{w}$ if we find $w>C/\lambda$ as follows
%\[	w(x, \epsilon)=\begin{cases}
%p(|x|+\epsilon)^{p-1}, &\text{ if } p(|x|+\epsilon)^{p-1}<C/\lambda\\
%\bar{w} &\text{ if } p(|x|+\epsilon)^{p-1}>C/\lambda
%\end{cases}
%\]

   	For the gradient with respect to  $\delta$, from   	$w\le C/\lambda$ by Theorem \ref{thm.stable.support}.
	\begin{equation}\label{eq:kl6}
 \|\nabla_\delta F(z^{k+1})\|_2  =	\|2\lambda   \delta^{k+1}\circ w^{k+1} \|_2  \leq  2 C \| \delta^{k+1}\|_2 
    =C_2\|\delta^{k+1}-\delta^k\|_2
 %  &:= C_2\|\delta^{k+1}-\delta^k\|_2
	\end{equation}
	with $C_2:=\frac{2C\sqrt{\mu}}{1-\sqrt{\mu} }$.
	Combine the above formulations \cref{eq:kl5} and \cref{eq:kl6},  yields  
	\begin{equation}
	\begin{aligned}
	\|\nabla  F(z^{k+1})\|_2 \leq &\ \|\nabla_x F(z^{k+1}) \|_2 + \|\nabla_\delta F(z^{k+1})\|_2 \\
	\leq &\ C_1 \|x^k-x^{k+1}\|_2 + C_2 \|\delta^{k+1}-\delta^{k}\|_2\\
	\leq &\ \max\{C_1, C_2\} (\|x^k-x^{k+1}\|_1+\|\delta^{k+1}-\delta^{k}\|_1)\\
	 = &\ \max\{C_1, C_2\}   \|z^k-z^{k+1}\|_1\\
	= &\ b \|z^k - z^{k+1}\|_2
	\end{aligned} 
	\end{equation}
	with $b:=\max\{C_1, C_2\} \sqrt{2n} $. 

	\textbf{C3.} This condition holds due to $F(x,\delta^2)$ is  continuous $\{z^k\}$ is bounded due to the Assumption of the coercivity of $F$. 
	
	Overall, we  have shown the sequence $\{(x^k,\delta^k)\}$ generated by \cref{alg.framework} satisfies the three conditions. The proof is completed.
\end{proof}
